# Supplementary material for: GeoTopoDiff: Learning Geometry--Topology Graph Priors through Boundary-Constrained Mixed Diffusion for Sparse-Slice 3D Porous Reconstruction
Source: arXiv:2605.03764 source file (2026-05-05)
Supplement: Supplementary file 1 [file appendix.tex]

\section{Additional experimental details}
\label{app:additional_results}

\subsection{Dataset statistics and preprocessing}

Table~\ref{tab:dataset_stats_app} summarizes the crop protocol used for the main experiments. The PTFE data are in-house micro-CT scans. For all datasets, the observed slices are the two boundary planes and the reconstruction target is the missing interior.

\begin{table}[h]
\caption{Dataset statistics and preprocessing.}
\label{tab:dataset_stats_app}
\centering
\begin{tabular}{lcccccc}
\toprule
Dataset & Phases & Raw size & Crop size & Train & Val & Test \\
\midrule
Fontainebleau & 2 & $762^3$ & $128^3$ & 1600 & 400 & 400 \\
PTFE fiber & 2 & $948^3$ & $128^3$ & 2000 & 600 & 600 \\
\bottomrule
\end{tabular}
\end{table}

\subsection{Metric definitions}

The two-point correlation function is computed for the pore indicator $I(x)$ as
\begin{equation}
S_2(r)=\mathbb P(I(x)=1,I(x+r)=1).
\end{equation}
PSD is computed from the distribution of pore diameters after binary segmentation. CDP is the empirical distribution of connected pore-cluster sizes under a fixed 3D voxel adjacency rule. Permeability is estimated from single-phase flow simulation using Darcy's law,
\begin{equation}
Q=\frac{K A\Delta P}{\mu L},
\end{equation}
where $K$ is permeability, $A$ is cross-sectional area, $\Delta P$ is pressure drop, $\mu$ is viscosity, and $L$ is the sample length.

\subsection{Additional morphology and topology curves}

\begin{figure}[h]
    \centering
    \todosmallfig{4_PSD.pdf}{0.9\linewidth}
    \caption{PSD relative error and KL divergence across training epochs. This diagnostic is moved to the appendix because the main paper emphasizes final reconstruction quality.}
    \label{fig:app_psd}
\end{figure}

\begin{figure}[h]
    \centering
    \todosmallfig{5_CDP.pdf}{0.9\linewidth}
    \caption{CDP comparison on Fontainebleau sandstone. \method{} better preserves connected pore-cluster distributions.}
    \label{fig:app_cdp}
\end{figure}

\subsection{Flow simulation visualization}

\begin{figure}[h]
    \centering
    \todofig{9_physics_simulation.pdf}{0.9\linewidth}
    \caption{PTFE air-flow simulation. The reconstructed velocity field from \method{} better preserves the dominant transport paths and high-velocity regions of the reference.}
    \label{fig:app_flow}
\end{figure}

\subsection{Full PTFE ablation table}

\begin{table}[h]
\caption{Full ablation results on anisotropic PTFE. Lower is better for all metrics.}
\label{tab:ablation_full_app}
\centering
\resizebox{\textwidth}{!}{%
\begin{tabular}{lccccccccc}
\toprule
Method & YZ RelErr & XZ RelErr & XY RelErr & YZ Var & XZ Var & XY Var & YZ KL & XZ KL & XY KL \\
\midrule
\method{} & \textbf{0.0089} & \textbf{0.0097} & \textbf{0.0068} & \textbf{0.0011} & \textbf{0.0012} & \textbf{0.0009} & \textbf{0.0043} & \textbf{0.0049} & \textbf{0.0035} \\
M1 & 0.0178 & 0.0186 & 0.0129 & 0.0026 & 0.0027 & 0.0019 & 0.0108 & 0.0112 & 0.0076 \\
M2 & 0.0143 & 0.0151 & 0.0108 & 0.0021 & 0.0023 & 0.0016 & 0.0084 & 0.0089 & 0.0061 \\
M3 & 0.0119 & 0.0127 & 0.0092 & 0.0017 & 0.0018 & 0.0013 & 0.0067 & 0.0071 & 0.0050 \\
M4 & 0.0108 & 0.0115 & 0.0084 & 0.0015 & 0.0016 & 0.0012 & 0.0058 & 0.0062 & 0.0044 \\
\bottomrule
\end{tabular}}
\end{table}

\begin{figure}[h]
    \centering
    \todofig{10_3D_view.pdf}{0.9\linewidth}
    \caption{Qualitative ablation on anisotropic PTFE. Removing graph conditioning or discrete topology diffusion increases fragmentation and boundary drift.}
    \label{fig:app_ablation_qual}
\end{figure}

\subsection{Robustness to observation sparsity}

\begin{figure}[h]
    \centering
    \todosmallfig{11_gap_plot.pdf}{0.9\linewidth}
    \caption{Robustness to observation sparsity. The reconstruction gap is varied over $M\in\{8,16,32,64,128,256\}$. The full model degrades more gracefully as the missing interval increases.}
    \label{fig:app_gap}
\end{figure}

\subsection{Sensitivity to boundary-graph quality}

\begin{table}[h]
\caption{Sensitivity to boundary-graph quality on Fontainebleau sandstone. Geometry jitter perturbs centroids by 1--2 voxels and radii by 5--10\%.}
\label{tab:graph_quality_app}
\centering
\begin{tabular}{lcccc}
\toprule
Setting & CDP KL $\downarrow$ & PR $\uparrow$ & Perm. RelErr $\downarrow$ & Bdry. Err $\downarrow$ \\
\midrule
Full graph & \textbf{0.00021} & \textbf{0.973} & \textbf{0.041} & \textbf{0.0001} \\
Nodes only (no edges) & 0.00079 & 0.892 & 0.087 & 0.0001 \\
10\% node dropout & 0.00036 & 0.948 & 0.053 & 0.0001 \\
20\% node dropout & 0.00058 & 0.921 & 0.068 & 0.0002 \\
5\% geom. jitter & 0.00031 & 0.956 & 0.049 & 0.0001 \\
10\% geom. jitter & 0.00047 & 0.934 & 0.061 & 0.0002 \\
\bottomrule
\end{tabular}
\end{table}

\subsection{Computing efficiency}

\begin{table}[h]
\caption{Relative computational efficiency of \method{} and ablated variants. Values are normalized by the full model. Lower is better.}
\label{tab:efficiency_app}
\centering
\begin{tabular}{lcccc}
\toprule
Method & Params & Peak GPU mem. & Train time/epoch & Sample time/vol. \\
\midrule
\method{} & 1.00 & 1.00 & 1.00 & 1.00 \\
M1 & 0.95 & 0.93 & 0.91 & 0.92 \\
M2 & \textbf{0.89} & \textbf{0.86} & \textbf{0.84} & \textbf{0.82} \\
M3 & 0.93 & 0.90 & 0.88 & 0.87 \\
M4 & 0.96 & 0.94 & 0.92 & 0.94 \\
\bottomrule
\end{tabular}
\end{table}
